# Supplementary material for: Cavity exciton-polaritons in two-dimensional semiconductors from first principles
Source: arXiv:2105.05591 ancillary file (2021-05-12)
Supplement: Supplementary file 1 [file Supp.pdf]

# Supplemental Material: Cavity exciton-polaritons in two-dimensional semiconductors from first principles

Dino Novko[1,2] and Vito Despoja[1,2,*]

[1] Institute of Physics, Bijenička 46, 10000 Zagreb, Croatia
[2] Donostia International Physics Center (DIPC), P. Manuel de Lardizabal, 4, 20018 San Sebastián, Spain

## S1. THEORETICAL FORMULATION

### A. Calculation of electrical field propagator $\mathcal{E}_{\mu\nu}$

The quantity from which we shall extract the informations about the electromagnetic modes in microcavity setup is electrical field propagator $\mathcal{E}_{\mu\nu}$. The electrical field produced by external oscillating point dipole $\mathbf{p}_0 e^{-i\omega t}$ placed in point $\mathbf{r}'$ is [S1]

$$E_\mu(\mathbf{r},\omega) = \sum_{\nu=x,y,z} \mathcal{E}_{\mu\nu}(\mathbf{r},\mathbf{r}',\omega) p^0_\nu, \qquad \text{(S1)}$$

Here the goal is to calculate the propagator $\mathcal{E}_{\mu\nu}$ in microcavity device which consists of substrate, tip and 2D crystal, described by local dielectric functions $\epsilon^+$, $\epsilon^-$ and conductivity tensor $\sigma_{\mu\nu}$, respectively. The substrate occupy region $z<0$, tip occupy region $z>d$, and the 2D crystal is immersed (at a height $z_0$ relative to the substrate) in dielectric media described by local dielectric function $\epsilon^0$ which occupies region $0<z<d$, as ilustrated in Fig.1 of the main text. The $\mathcal{E}_{\mu\nu}$ can be connected with the time-ordered photon propagator $D_{\mu\nu} = \frac{i}{\hbar c}\langle T\{A_\mu A_\nu\}\rangle$ as $\mathcal{E}_{\mu\nu} = \frac{i\omega}{c} D_{\mu\nu}$. Due to the aforesaid, the electric field propagator satisfies the Dyson equation $\mathcal{E} = \Gamma + \Gamma\sigma\mathcal{E}$, where $\Gamma$ represents the propagator of electrical field in the absence of 2D crystal, i.e. when $\sigma = 0$ [S2, S3]. After imposing the planar symmetry of the microcavity device the Dyson equation for propagator $\mathcal{E}$ becomes explicitly

$$\begin{aligned}\mathcal{E}_{\mu\nu}(\mathbf{Q},\omega,z,z') = \Gamma_{\mu\nu}(\mathbf{Q},\omega,z,z') + \\ \sum_{\alpha,\beta=x,y,z}\int_{-\infty}^{\infty} dz_1 \int_{-\infty}^{\infty} dz_2\, \Gamma_{\mu\alpha}(\mathbf{Q},\omega,z,z_1)\times \\ \sigma_{\alpha\beta}(\mathbf{Q},\omega,z_1,z_2)\mathcal{E}_{\beta\nu}(\mathbf{Q},\omega,z_2,z'),\end{aligned} \qquad \text{(S2)}$$

where $\mathbf{Q} = (Q_x,Q_y)$ and $\omega$ are transfer wave-vector and frequency, respectively. The propagator of electrical field, in absence of 2D crystal can be written as

$$\mathbf{\Gamma} = \mathbf{\Gamma}^0 + \mathbf{\Gamma}^{sc}, \qquad \text{(S3)}$$

where the propagator of 'free' electrical field (or free photons propagator) is [S1, S2]

$$\begin{aligned}\mathbf{\Gamma}^0(\mathbf{Q},\omega,z,z') = -\frac{4\pi}{\epsilon^0}\delta(z-z')\mathbf{z}\cdot\mathbf{z} + \\ \frac{2\pi i\omega^2}{\beta^0 c^2}\left\{\mathbf{e}^0_s\cdot\mathbf{e}^0_s + \mathbf{e}^0_p\cdot\mathbf{e}^0_p\right\} e^{i\beta^0|z-z'|}.\end{aligned} \qquad \text{(S4)}$$

The propagator of scattered electrical field in region $0<z<d$, which describes multiple reflections of electromagnetic field at the microcavity interfaces [S1] [see also Fig. 2(b) of the main text], is

$$\begin{aligned}\mathbf{\Gamma}^{sc}(\mathbf{Q},\omega,z,z') = \frac{2\pi i\omega^2}{\beta^0 c^2}\frac{1}{D_q}\Big\{r^-_q e^{i\beta^0(z+z')}\cdot\mathbf{e}^+_q\cdot\mathbf{e}^-_q + \\ r^-_q r^+_q e^{i\beta^0(z-z'+2d)}\cdot\mathbf{e}^+_q\cdot\mathbf{e}^+_q + r^+_q e^{-i\beta^0(z+z'-2d)}\cdot\mathbf{e}^-_q\cdot\mathbf{e}^+_q + \\ r^-_q r^+_q e^{-i\beta^0(z-z'-2d)}\cdot\mathbf{e}^-_q\cdot\mathbf{e}^-_q\Big\};\ \text{q=s(TE), p(TM)}.\end{aligned} \qquad \text{(S5)}$$

Here $D_q = 1 - r^-_q r^+_q e^{2i\beta^0 d}$. The unit vectors of $\mathbf{s}$(TE) polarised electromagnetic field are

$$\mathbf{e}^{0,\pm}_s = \mathbf{Q}_0\times\mathbf{z},$$

and the unit vectors of $\mathbf{p}$(TM) polarised electromagnatic field are

$$\mathbf{e}^{0,\pm}_p = \frac{c}{\omega\sqrt{\epsilon^0}}\left[\alpha^{0,\pm}\beta^0\mathbf{Q}_0 + Q\mathbf{z}\right],$$

where $\alpha^0 = -sgn(z-z')$, $\alpha^\pm = \mp 1$, and $\mathbf{Q}_0$ and $\mathbf{z}$ are unit vectors in $\mathbf{Q}$ and $z$ directions, respectively. The reflection coefficients of s(TE) and p(TM) polarised electromagnetic waves at media/substrate (-) and and media/tip (+) interfaces are

$$r^\pm_s = \frac{\beta^0-\beta^\pm}{\beta^0+\beta^\pm} \qquad \text{(S6)}$$

and

$$r^\pm_p = \frac{\beta^0\epsilon^\pm-\beta^\pm\epsilon^0}{\beta^0\epsilon^\pm+\beta^\pm\epsilon^0}, \qquad \text{(S7)}$$

respectively. The complex wave vectors in perpendicular ($z$) direction are

$$\beta^{0,\pm} = \sqrt{\frac{\omega^2}{c^2}\epsilon^{0,\pm}(\omega) - Q^2}. \qquad \text{(S8)}$$

In order to simplify the interpretation of the results, in the main text we suppose that the dielectric media is vacuum, i.e. $\epsilon^0 = 1$. In addition, we suppose

*Electronic address: vdespoja@ifs.hr

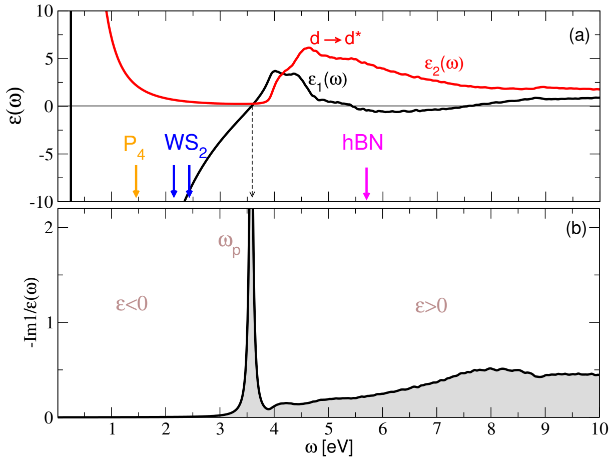


FIG. S1: (a) Silver macroscopic dielectric function and (b) energy loss function. Wave vector is $Q = 0.017\,$a.u. The arrows denote the exciton energies in phosphorene $P_4$, $WS_2$, and hBN.

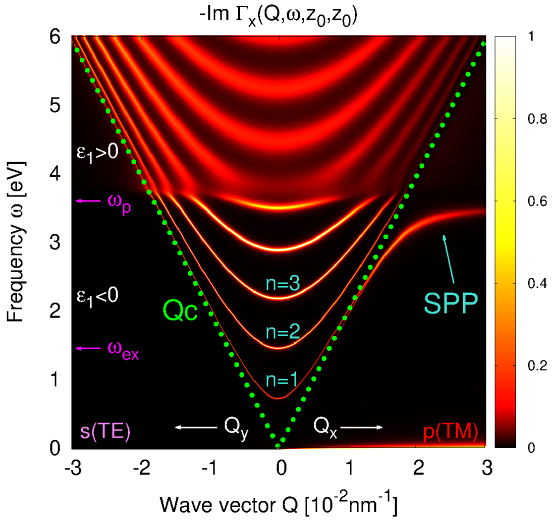


FIG. S2: The intensity of electromagnetic modes in silver planar cavity. The silver surfaces are separated by distance $d = 800\,$nm and $z_0 = 50\,$nm. The arrows denote the phosporene exciton at $\hbar\omega_{ex} = 1.45\,$eV and silver plasmon at $\hbar\omega_p$=3.6 eV.

that tip and substrate are made of the same material, i.e. $\epsilon^- = \epsilon^+ = \epsilon$. Preferably, this material should be highly reflective, so we shall assume here that the substrate and tip are made of silver or aluminium. Figure S1 shows silver (a) macroscopic dielectric function $\epsilon(\omega)$ and (b) Energy Loss Function (ELF). The wave vector is $Q = 0.017\,$a.u., the minimum wave vector allowed by Brillouin zone (BZ) sampling. Besides the interband $d \to p^*$ and $p \to s^*$ transitions (onset at about 4eV in $\epsilon_2$) the silver behaves as a Drude metal supporting bulk plasmon at $\omega_p \approx 3.6\,$eV. Therefore we have that $\epsilon_1(\omega < \omega_p) < 0$ and $\epsilon_1(\omega > \omega_p) > 0$. Consequently, e.g. for $Q = 0$ and $\omega < \omega_p$, the $\beta^\pm = \frac{\omega}{c}\sqrt{\epsilon(\omega)} \in \mathbb{C}$, which means the electromagnetic field has evanescent character inside the substrate or tip, and the reflection at the surfaces is efficient. On the contrary, for $\omega > \omega_p$ the electromagnetic field has radiative character inside the substrate or tip, and the reflection is less efficient. From the results presented in Fig. S1(a) it is obvious that in the frequency region of phosphorene exciton or $WS_2$ A and B excitons (denoted by arrows) the $\epsilon_1$ is large negative number so that the silver surfaces is there highly reflective. However, the energy of hBN exciton is larger than silver plasmon so in order to ensure good reflectivity in that case, silver will be replaced by aluminum, for which $\omega_p \approx 15\,$eV.

The poles of propagator $\Gamma$ or zeros of its denominator

$$D_q = 0,\ \ q = s, p, \tag{S9}$$

determines the dispersion relations of electromagnatic eigenmodes supported by microcavity. If the $\epsilon_1$ is large negative number, according to Eqs.S6 and S7 the reflectivities can be approximated as $r_{s,p} \approx \mp 1$ (limit of perfect reflectivity) and the Eq.S9 reduces to $e^{2i\beta^0 d} = 1$ which in radiative region ($\omega > Qc$) leads to dispersion relations of cavity-modes

$$\omega_n^0(Q) = c\sqrt{\frac{n^2\pi^2}{d^2} + Q^2},\ \ n = 1, 2, 3, ... \tag{S10}$$

Figure S2 show the intensity of electromagnetic modes $-\mathrm{Im}\,\Gamma(\mathbf{Q}, \omega, z_0, z_0)$ in silver planar cavity of thickness $d = 800$nm and $z_0 = 50$nm. It can bi notice that the cavity modes are well defined in region $\omega < \omega_p$, while in region $\omega > \omega_p$ becomes dispersive. The surface plasmon polariton (SPP) in evanescent region ($\omega < Qc$) is also visible. First few cavity modes $\omega_n(Q = 0) \sim$ 0.74, 1.47, 2.2 eV lie in region of strong reflectivity and agrees well with the values obtained with the simple formula (S10) $\omega_n^0(Q) = 0.78,\ 1.55,\ 2.33\,$eV.

Since we are here interested in the electromagnatic modes in the visible and UV frequency regions, i.e., $\hbar\omega <$ 6 eV, according to formula (S8), the maximum wavelength in parallel or perpendicular direction $\lambda^0 = 2\pi c/\omega$ is incomparably larger than the 2D crystal thickness and unite cell. Consequently, the dynamical response of 2D crystal can be can be approximated by local 2D optical conductivity

$$\sigma_{\mu\nu}(\mathbf{Q}, \omega, z, z') \approx \sigma_{\mu\nu}(\omega)\delta_{\mu\nu}\delta(z - z_0)\delta(z' - z_0). \tag{S11}$$

After using this approximation, the equation (S2) reduces to matrix equation for the electrical field propagator in the vicinity of the 2D crystal ($z = z' = z_0$)

$$\mathcal{E}_{\mu\nu}(\mathbf{Q}, \omega, z_0, z_0) = \Gamma_{\mu\nu}(\mathbf{Q}, \omega, z_0^+, z_0) + \sum_{\alpha=x,y,z} \Gamma_{\mu\alpha}(\mathbf{Q}, \omega, z_0^+, z_0)\sigma_\alpha(\omega)\mathcal{E}_{\alpha\nu}(\mathbf{Q}, \omega, z_0, z_0). \tag{S12}$$

Here we put $z_0^+ = z_0 + \delta$, where $\delta > 0$ is infinitesimally small number, in order to eliminate local term in $\Gamma^0_{zz}$.

### B. Calculation of optical conductivity $\sigma_\mu(\omega)$

The optical conductivity is calculated beyond the random phase approximation (RPA), i.e. the RPA optical conductivity is corrected by the ladder term

$$\sigma_\mu(\omega) = \sigma_\mu^{RPA}(\omega) + \sigma_\mu^{ladd}(\omega), \tag{S13}$$

as ilustrated by Feynman diagrams in Fig. S3(a). It is also useful to divide the RPA optical conductivity to its intra- and inter-band contributions

$$\sigma_\mu^{RPA}(\omega) = \sigma_\mu^{\text{intra}}(\omega) + \sigma_\mu^{\text{inter}}(\omega), \tag{S14}$$

such that total conductivity reads

$$\sigma_\mu(\omega) = \sigma_\mu^{\text{intra}}(\omega) + \sigma_\mu^{\text{inter}}(\omega) + \sigma_\mu^{ladd}(\omega). \tag{S15}$$

The local conductivities are determined from optical limit of nonlocal conductivities $\sigma^i_\mu(\omega) = \sigma^i_\mu(\omega, \mathbf{Q} \approx 0)$ where the RPA intraband ($n = m$) conductivity is [S3]

$$\sigma_\mu^{\text{intra}}(\mathbf{Q},\omega) = i\frac{e^2}{m}\frac{n_\mu}{\omega + i\eta_{intra}}. \tag{S16}$$

Here the effective number of charge carriers is

$$n_\mu = -\frac{m}{Se^2}\sum_n\sum_{\mathbf{K}\in 1.SBZ}\frac{\partial f_{n\mathbf{K}}}{\partial E_{n\mathbf{K}}}\left|j^\mu_{n\mathbf{K},n\mathbf{K}}\right|^2. \tag{S17}$$

The interband ($n \neq m$) conductivity is [S3]

$$\sigma_\mu^{\text{inter}}(\mathbf{Q},\omega) = -\frac{i\hbar}{S}\sum_{n\neq m}\sum_{\mathbf{K}\in 1.S.B.Z.}\frac{\left|j^\mu_{n\mathbf{K},m\mathbf{K}+\mathbf{Q}}\right|^2}{E_{n\mathbf{K}} - E_{m\mathbf{K}+\mathbf{Q}}}\times \frac{f_{n\mathbf{K}} - f_{m\mathbf{K}+\mathbf{Q}}}{\hbar\omega + i\eta_{inter} + E_{n\mathbf{K}} - E_{m\mathbf{K}+\mathbf{Q}}}. \tag{S18}$$

Here the curent vertices are

$$j^\mu_{n\mathbf{K},m\mathbf{K}+\mathbf{Q}} = \int_\Omega d\mathbf{r} e^{-i\mathbf{Q}\mathbf{r}}\, j^\mu_{n\mathbf{K},m\mathbf{K}+\mathbf{Q}}(\mathbf{r}), \tag{S19}$$

where the current produced by transitions between Bloch states $\phi^*_{n\mathbf{K}} \to \phi_{m\mathbf{K}+\mathbf{Q}}$ are defined as

$$j^\mu_{n\mathbf{K},m\mathbf{K}+\mathbf{Q}}(\mathbf{r}) = \frac{e\hbar}{2im}\left\{\phi^*_{n\mathbf{K}}(\mathbf{r})\partial_\mu\phi_{m\mathbf{K}+\mathbf{Q}}(\mathbf{r}) - [\partial_\mu\phi^*_{n\mathbf{K}}(\mathbf{r})]\phi_{m\mathbf{K}+\mathbf{Q}}(\mathbf{r})\right\}.$$

The 2D wave vectors are $\mathbf{K} = (K_x, K_y)$, while $\phi_{n\mathbf{K}}$ and $E_{n\mathbf{K}}$ are Bloch wave functions and energies obtained in the DFT calculations. Considering that we study the 2D semiconductors, the energies $E_{n\mathbf{K}}$ are also corrected using the GW method. The spin quantum number $s$ is merged with bands quantum number, i.e. $n \equiv (n, s)$, $\Omega =$ $S \times L$ is the normalization volume, $S$ is the normalization surface and $f_{n\mathbf{K}} = [e^{(E_{n\mathbf{K}}-E_F)/kT} + 1]^{-1}$ is the Fermi-Dirac distribution function at the temperature $T$. The ladder contribution to conductivity is

$$\sigma_\mu^{ladd}(\mathbf{Q},\omega) = \frac{i}{\omega S}\sum_{nm\mathbf{K}}\sum_{n'm'\mathbf{K}'} j^\mu_{n\mathbf{K},m\mathbf{K}+\mathbf{Q}} \times \mathcal{K}^{m\mathbf{K}+\mathbf{Q}\leftarrow m'\mathbf{K}'+\mathbf{Q}}_{n\mathbf{K}\to n'\mathbf{K}'}(\omega)[j^\mu_{n'\mathbf{K}',m'\mathbf{K}'+\mathbf{Q}}]^*, \tag{S20}$$

where ladder 4-point polarizability $\mathcal{K}$ can be obtained by solving the matrix equation in the $(\mathbf{K}, n)$-space, i.e.,

$$\mathcal{K}(\omega) = \mathcal{L}(\omega)\otimes\Phi^F\otimes\mathcal{L}(\omega) + \mathcal{L}(\omega)\otimes\Phi^F\otimes\mathcal{K}(\omega), \tag{S21}$$

where matrix multiplication represents next summation over the bands and wave vectors $\otimes \equiv \sum_{nm}\sum_{\mathbf{K}}$. Here the time-ordered electron-hole propagator is explicitly

$$\mathcal{L}^{m\mathbf{K}+\mathbf{Q}\leftarrow m'\mathbf{K}'+\mathbf{Q}}_{n\mathbf{K}\to n'\mathbf{K}'} = \delta_{nn'}\delta_{mm'}\delta_{\mathbf{K}\mathbf{K}'}\times \left\{\frac{f_{n\mathbf{K}}(1-f_{m\mathbf{K}+\mathbf{Q}})}{\omega + E_{n\mathbf{K}} - E_{m\mathbf{K}+\mathbf{Q}} + i\delta} - \frac{f_{m\mathbf{K}+\mathbf{Q}}(1-f_{n\mathbf{K}})}{\omega + E_{n\mathbf{K}} - E_{m\mathbf{K}+\mathbf{Q}} - i\delta}\right\},$$

and the Bethe-Salpeter-Fock kernel is

$$\Phi^{F,m\mathbf{K}+\mathbf{Q}\leftarrow m'\mathbf{K}'+\mathbf{Q}}_{n\mathbf{K}\to n'\mathbf{K}'} = -\frac{1}{\Omega}\rho^*_{n\mathbf{K},n'\mathbf{K}'}W^T(\mathbf{K}'-\mathbf{K},\omega=0)\rho_{m\mathbf{K}+\mathbf{Q},m'\mathbf{K}'+\mathbf{Q}}, \tag{S22}$$

where the charge vertices are

$$\rho_{n\mathbf{K},m\mathbf{K}+\mathbf{Q}} = \int_\Omega d\mathbf{r}\, \phi^*_{n\mathbf{K}}(\mathbf{r})e^{-i\mathbf{Q}\mathbf{r}}\phi_{m\mathbf{K}+\mathbf{Q}}(\mathbf{r}). \tag{S23}$$

The RPA time-ordered screened Coulomb interaction is

$$W^T(\mathbf{Q},\omega) = v_Q/\epsilon(\mathbf{Q},\omega), \tag{S24}$$

where $v_Q = 2\pi/Q$, the longitudinal 2D dielectric function is

$$\epsilon(\mathbf{Q},\omega) = 1 - v_Q\chi^0(\mathbf{Q},\omega), \tag{S25}$$

and the time-ordered response function is

$$\chi^0(\mathbf{Q},\omega) = \frac{1}{S}\sum_{nm\mathbf{K}}\left|\rho_{n\mathbf{K},m\mathbf{K}+\mathbf{Q}}\right|^2\times \frac{(f_{n\mathbf{K}} - f_{m\mathbf{K}+\mathbf{Q}})}{\hbar\omega + E_{n\mathbf{K}} - E_{m\mathbf{K}+\mathbf{Q}} + i\delta sgn(E_{m\mathbf{K}+\mathbf{Q}} - E_{n\mathbf{K}})}. \tag{S26}$$

This 'RPA+ladder' approach is equivlent to widely used time-dependent screened Hartree-Fock (TDSHF) approximation [S4–S11]. Also, here the interaction between the electrons and holes, $W^T$ in Fock-kernel (S22), is not corrected by the presence of a microcavity. This is a reasonable approximation because the cavity-photons (far-field) weakly affect the exciton binding energy. Note that the

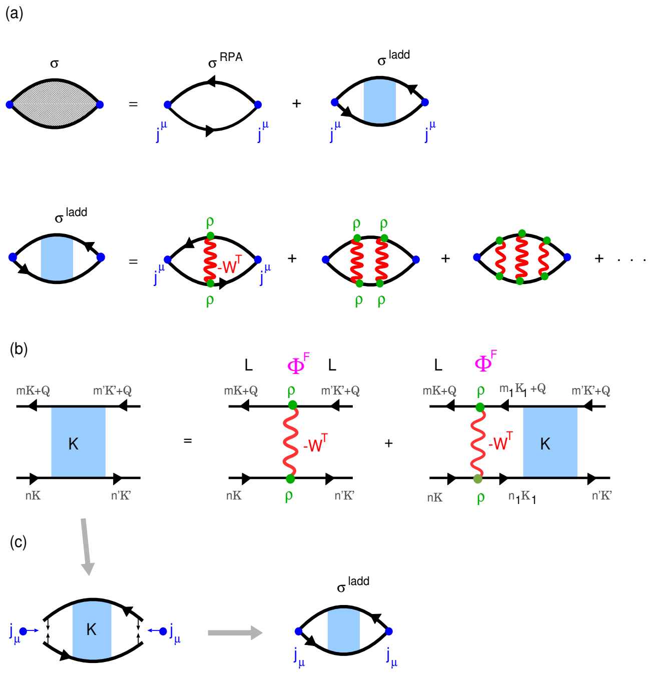


FIG. S3: (a) Feynman diagrams representing the optical conductivity $\sigma_\mu$ and the perturbative expansion of the ladder contribution to the optical conductivity $\sigma_\mu^{ladd}(\omega)$. (b) The matrix equation for the ladder 4-point polarizability $\mathcal{K}$. (c) The ladder optical conductivity $\sigma_\mu^{ladd}(\omega)$ is obtained such that in $\mathcal{K}$ the fermionic lines are first contracted and multiplied by corresponding current vertices $j^\mu$. Then summations over the bands and wave vectors are performed, i.e., $\sigma_\mu^{ladd}(\mathbf{Q},\omega) = \frac{i}{\omega S}\sum_{nm\mathbf{K}}\sum_{n'm'\mathbf{K}'} j^\mu\ \mathcal{K}\ [j^\mu]^*$. Blue dots represent the current vertices $j^\mu$, green dots represents the charge vertices $\rho$ and red wavy lines represent the screened Coulomb interaction $W^T$.

evanescent SPP might affect the exciton binding energy, however, this issue will not be examined here. The calculation of 'ladder' optical conductivity $\sigma^{ladd}$ is summarised by Feynman diagrams in Figs. S3(b) and S3(c). First, the ladder 4-point polarizability $\mathcal{K}$ is obtained by solving the matrix equation shown in Fig. S3(b). Second, in $\mathcal{K}$ the fermionic lines are first contracted and multiplied by the corresponding current vertices $j^\mu$ and finally summations over the bands and wave vectors are performed, as illustrated in Fig. S3(c).

Figures S4(a) and S4(b) show the real parts of optical conductivities in phosporene calculated using RPA+ladder method for the two in-plane polarization directions, i.e., Re$\sigma_x$ and Re$\sigma_y$. The RPA optical conductivities are also shown for the comparison. The obtained phosporene GW band gap used in this calculation is $E_g = 2.05\,$eV. In Re$\sigma_x$ we observe a strong exciton at $\hbar\omega_{ex} = 1.45\,$eV, with the binding energy of about $\Delta = E_g - \hbar\omega_{ex} = 600\,$meV. The phosphorene absorption is strongly anisotropic so that the exciton does not appear in Re$\sigma_y$, as it was already theoretically and experimentaly confirmed [S12–S17].

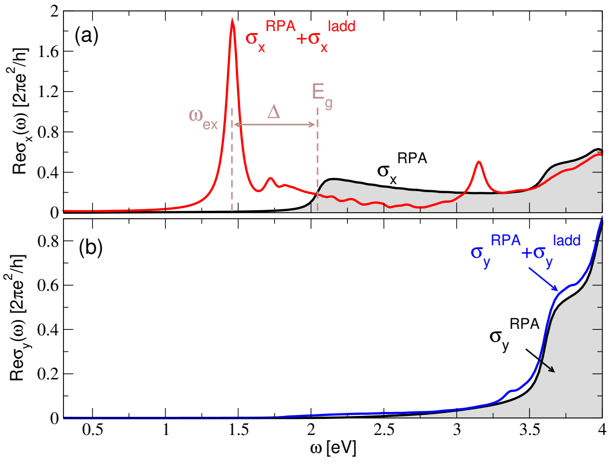


FIG. S4: The real parts of phosphorene optical conductivities (a) Re$\sigma_x(\omega)$ and (b) Re$\sigma_y(\omega)$. The RPA optical conductivites (shaded area) are also shown for the comparison.

Figures S5 depict the Re$\sigma_x(\omega)$ in (a) hBN and (b) $WS_2$ calculated by means of the 'RPA+ladder' method. The RPA optical conductivities are also shown for the comparison. For the hBN and $WS_2$ band gap we use $E_g = 7.48\,$eV and $E_g = 2.7\,$eV, respectively (which was also obtained with the GW method). The hBN monolayer supports strong exciton at $\hbar\omega_{ex} = 5.67\,$eV whose binding energy is $\Delta = E_g - \hbar\omega_{ex} = 1.72\,$eV. The latter agrees well with the value of $\Delta = 1.89\,$eV reported, e.g., in Ref. [S18]. The $WS_2$ supports two spin-orbit splitted excitons A and B at $\hbar\omega_{ex}^A = 2.1\,$eV and $\hbar\omega_{ex}^B = 2.46\,$eV. The binding energy of A exciton is $\Delta = 0.6\,$eV which agrees well with theoretical and experimental value $\Delta = 0.7$eV reported in Refs. [S19, S20]

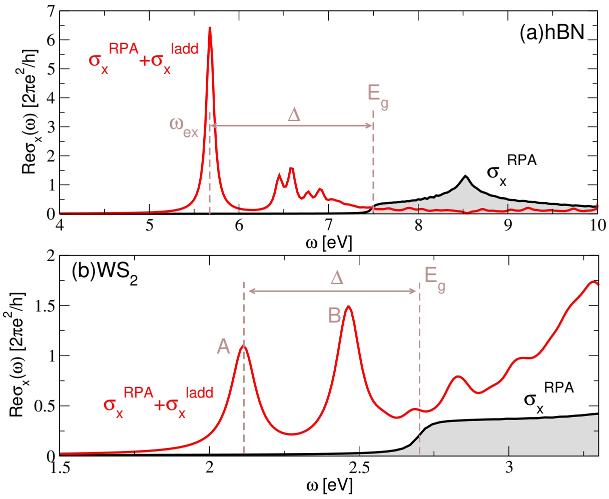


FIG. S5: (a) The real parts of optical conductivities Re$\sigma_x(\omega)$ in the (a) hBN and in (b) $WS_2$ monolayers. The RPA optical conductivites (shaded areas) are also shown for the comparison.

## S2. COMPUTATIONAL DETAILS

### A. Ground state calculations

The KS wave functions $\phi_{n\mathbf{K}}$ and energies $E_{n\mathbf{K}}$ used to calculate the 'RPA+ladder' conductivities $\sigma$ and metallic macroscopic dielectric functions $\epsilon(\omega)$ were determined using a plane-wave self-consistent field DFT code (PWSCF) within the QUANTUM ESPRESSO (QE) package [S21]. For all the crystal structures studied in the present work (phosphorene $P_4$, $WS_2$, and hBN single layers, as well as bulk Ag and bulk Al) the core-electrons interaction was approximated by the norm-conserving pseudopotentials [S22, S23]. The exchange correlation (XC) potentials in $P_4$ and Ag were approximated by the scalar-relativistic and in $WS_2$ by the fully-relativistic Perdew-Burke-Ernzerhof (PBE) generalized gradient approximation (GGA) functional [S24]. In Al an hBN the XC potentials were approximated by the Perdew-Zunger (PZ) local density approximation (LDA) functional [S25]. For $P_4$ the ground state electronic density was calculated by using the $26 \times 37 \times 1$ Monkhorst-Pack K-mesh [S26], the plane-wave cut-off energy was 50 Ry, the used Bravais lattice was orthorhombic, where $a = 4.631$ Å and $b = 3.3062$ Å, and the separation between the adjacent $P_4$ monolayers in the supercell was $L = 4a$. For hBN and $WS_2$ the ground state electronic densities were calculated using the $12 \times 12 \times 1$ K-mesh, the plane-wave cut-off energy was 60 Ry, the used Bravais lattices were hexagonal, where $a = 2.511$ Å and $a = 3.186$ Å, respectively, and the separation between MLs in a supercell was $L = 5a$. The ground state electronic densities of bulk Al and Ag crystals were calculated by using the $8 \times 8 \times 8$ K-mesh and the crystal structures were simulated by cubic FCC with lattice constants $a = 4.05$ Å and $a = 4.143$ Å, respectively. The used plane-wave cut-off energy was 80 Ry.

### B. Calculation of optical conductivity $\sigma_\mu$

The wave vector $\mathbf{K}$ summations in RPA optical conductivities (S16)–(S19) and screened Coulomb interactions (S24)–(S26) were performed by using the $201 \times 201 \times 1$ K-mesh for hBN and $WS_2$ and using the $109 \times 151 \times 1$ K-mesh for $P_4$. The band summations were performed over 50 bands in hBN and over 100 bands in $WS_2$ and $P_4$. The dimension of the $\{\mathbf{K}, n\}$-space used to calculate the BSE-Fock kernels (S22), the 4-point polarisability matrices (S21) and finally the ladder optical conductivities (S20) in hBN and $WS_2$ consisted of $51 \times 51 \times 1$ K-points and in $P_4$ of $53 \times 75 \times 1$ K-points as well as two (one valence and one conduction) bands. The crystal local field effects LFE were not included in the calculations. The energies $E_{n\mathbf{K}}$ used to claculate RPA+ladder conductivities were corrected using the GW quasiparticle approximation as implemented within the real space projector augmented wavefunction (PAW) code GPAW [S27, S28]. The corresponding ground state parameters and crystal structures were as in the QE calculations. Also, for hBN and $WS_2$ we have used the $36 \times 36 \times 1$ while for $P_4$ the $20 \times 30 \times 1$ K-grid. The number of the bands for the GW calculates were 100 for all three monolayers and the energy cutoff for the local field effect vectors was 80 eV. The self-consistent GW0 method with $n = 3$ steps was used.

### C. Calculation of macroscopic dielectric function $\epsilon(\omega)$

In the main text we suppose that the dielectric media is vacuum $\epsilon^0 = 1$, and that the substrate and tip are made from the same higly reflective material so that $\epsilon^-(\omega) = \epsilon^+(\omega) = \epsilon(\omega)$, where $\epsilon(\omega)$ represents the macroscopic dielectric function of silver or aluminium. The 3D Fourier transform of independent electrons response function is given by

$$\chi^0_{\mathbf{G}\mathbf{G}'}(\mathbf{q},\omega) = \frac{2}{\Omega}\sum_{n,m,\mathbf{k}} \rho_{n\mathbf{k},m\mathbf{k}+\mathbf{q}}(\mathbf{G})\ \rho^*_{n\mathbf{k},m\mathbf{k}+\mathbf{q}}(\mathbf{G}')\times \frac{f_n(\mathbf{k}) - f_m(\mathbf{k}+\mathbf{q})}{\omega + i\eta + E_n(\mathbf{k}) - E_m(\mathbf{k}+\mathbf{q})}, \tag{S27}$$

where the charge vertices are defined as

$$\rho_{n\mathbf{k},m\mathbf{k}+\mathbf{q}}(\mathbf{G}) = \int_\Omega d\mathbf{r}\ \phi^*_{n\mathbf{k}}(\mathbf{r}) e^{-i(\mathbf{q}+\mathbf{G})\mathbf{r}} \phi_{m\mathbf{k}+\mathbf{q}}(\mathbf{r}), \tag{S28}$$

and here $\mathbf{k} = (k_x, k_y, k_z)$, $\mathbf{q} = (q_x, q_y, q_z)$ and $\mathbf{G} = (G_x, G_y, G_z)$ are 3D the wave vector, transfer wave vector and reciprocal lattice vector, respectively. The integration is performed over the normalization volume $\Omega$. From response matrix (S27) we determine the dielectric matrix

$$\mathcal{E}_{\mathbf{G}\mathbf{G}'}(\mathbf{q},\omega) = \delta_{\mathbf{G}\mathbf{G}'} - \sum_{\mathbf{G}_1} v_{\mathbf{G}\mathbf{G}_1}(\mathbf{q}) \chi^0_{\mathbf{G}_1\mathbf{G}'}(\mathbf{q},\omega), \tag{S29}$$

where bare Coulomb interaction is $v_{\mathbf{G}\mathbf{G}'}(\mathbf{q}) = \frac{4\pi}{|\mathbf{q}+\mathbf{G}|^2}\ \delta_{\mathbf{G}\mathbf{G}'}$. Finally the macroscopic dielectric function is determined by inverting the dielectric matrix

$$\epsilon(\omega) = \epsilon_1(\omega) + i\epsilon_2(\omega) = 1/\mathcal{E}^{-1}_{\mathbf{G}=0\mathbf{G}'=0}(\mathbf{q}\approx 0,\omega). \tag{S30}$$

The ELF, in the optical limit, can be expressed in terms of macroscopic dielectric function as

$$P(\mathbf{q}\approx 0,\omega) \propto -\mathrm{Im}\,\frac{1}{\epsilon(\omega)}. \tag{S31}$$

The wave vector $\mathbf{k}$ summations in the response functions (S27) are performed using $41 \times 41 \times 41$ and $81 \times 81 \times 81$ $k$-meshes for Al and Ag, respectively. The band summations $(n, m)$ are performed over 20 and 33 bands for Al and Ag, respectively. The damping parameters are $\eta = 100$ meV and 40 meV for Al and Ag, respectively, and temperature is $T = 10$ meV. For optically small wave vectors ($\mathbf{q} \approx 0$), used in this modeling, the crystal local field effects are negligible, so the cuttoff energy of crystal local field effects is set to be zero.

[S1] M. S. Tomaš, Phys. Rev. A **51**, 2545 (1995)
[S2] V. Despoja, M. Šunjić, L. Marušić, Phys. Rev. B **80**, 075410 (2009).
[S3] D. Novko, M. Šunjić, V. Despoja, Phys. Rev B **93**, 125413 (2016)
[S4] L. Hedin, Phys. Rev. **139**, A796 (1965)
[S5] W. Hanke and L. J. Sham, Phys. Rev. Lett. **43**, 387 (1979)
[S6] W. Hanke and L. J. Sham, Phys. Rev. B **21**, 4656 (1980)
[S7] G. Strinati, Phys. Rev. B **29**, 5718 (1984)
[S8] M. S. Hybertsen, S. G. Louie, Phys. Rev. B **34**, 5390 (1986). [85] M. Rohlfing, S. G. Louie, Phys. Rev. Lett. **81**, 2312 (1998)
[S9] M. Rohlfing and S. G. Louie, Phys. Rev. Lett. **83**, 856 (1999)
[S10] M. Rohlfing, S. G. Louie, Phys. Rev. B **62**, 4927 (2000).
[S11] G. Onida, L. Reining, A. Rubio, Rev. Mod. Phys. **74**, 601 (2002).
[S12] F. Ferreira and R. M. Ribeiro, Phys. Rev B **96**, 115431 (2017)
[S13] C. E. P. Villegas, A. S. Rodin, A. C. Carvalho, and A. R. Rocha, Physical Chemistry Chemical Physics **18** (40) (2016)
[S14] R. Tian, R. Fei, S. Hu, T. Li, B. Zheng, Y. Shi, J. Zhao, L. Zhang, X. Gan and X. Wang, Phys. Rev. B **101**, 235407 (2020)
[S15] X. Wang, A. M. Jones, K. L. Seyler, V. Tran, Yichen Jia, Huan Zhao, Han Wang, Li Yang, Xiaodong Xu and Fengnian Xia, Nature Nanotechnology **10**, 517 (2015)
[S16] J. Yang, R. Xu, J. Pei, Ye Win Myint, F. Wang, Z. Wang, S. Zhang, Z. Yu and Yuerui Lu, Light: Science & Applications **4**, 312 (2015)
[S17] Likai Li, J. Kim, C. Jin, G. Jun Ye, D. Y. Qiu, F. H. da Jornada, Z. Shi, L. Chen, Z. Zhang, F. Yang, K. Watanabe, T. Taniguchi, W. Ren, S. G. Louie, X. Hui Chen, Y. Zhang, and Feng Wang, Nature Nanotechnology **12**, 21 (2017)
[S18] J. Yan, K. W. Jacobsen, K. S. Thygesen, Phys. Rev. B **86**, 045208 (2012)
[S19] Ziliang Ye, Ting Cao, Kevin O'Brien, Hanyu Zhu, Xiaobo Yin, Yuan Wang, Steven G. Louie and Xiang Zhang, Nature **513**, 214 (2014)
[S20] B. Zhu, X. Chen and X. Cui, Scientific Reports **5**, 9218 (2015)
[S21] P. Giannozzi, S. Baroni, N. Bonini, M. Calandra, R. Car, C. Cavazzoni, D. Ceresoli, G. L. Chiarotti, M. Cococcioni, I. Dabo, *et.al.*, J. Phys.: Conden. Matter **21**, 395502 (2009)
[S22] N. Troullier and J. L. Martins, Phys. Rev. B **43**, 1993 (1991)
[S23] D. R. Hamann, Phys. Rev. B **88**, 085117 (2013)
[S24] J. P. Perdew, K. Burke, and M. Ernzerhof, Phys. Rev. Lett. **77**, 3865 (1996)
[S25] J.P. Perdew and A. Zunger, Phys. Rev. B **23**, 5048 (1981)
[S26] H.J. Monkhorst and J.D. Pack, Phys. Rev. B **13**, 5188 (1976)
[S27] J. J. Mortensen, L. B. Hansen, and K. W. Jacobsen, Phys. Rev. B **71**, 035109 (2005).
[S28] J. Enkovaara, C. Rostgaard, J. J. Mortensen, J. Chen, M. Dulak, L. Ferrighi, J. Gavnholt, C.f Glinsvad, V. Haikola, H. A. Hansen, H. H. Kristoffersen, M. Kuisma, A. H. Larsen, L. Lehtovaara, M. Ljungberg, O. Lopez-Acevedo, P. G. Moses, J. Ojanen, T. Olsen, V. Petzold, N. A. Romero, J. Stausholm-Moller, M. Strange, G. A. Tritsaris, M. Vanin, M. Walter, B. Hammer, H. Hakkinen, G. K. H. Madsen, R. M. Nieminen, J. K. Norskov, M. Puska, T. T. Rantala, J. Schiotz, K. S. Thygesen, and K. W. Jacobsen, J. Phys.: Condens. Matter **22**, 253202 (2010).
